# Supplementary material for: Glyph-Based Uncertainty Visualization and Analysis of Time-Varying Vector Fields
Source: arXiv:2409.00042 source file (2024-08-18)
Supplement: Supplementary file 1 [file appendix.tex]

% \newpage
% \section{extra}
% \tajo{The text and figures below are added for discussion purposes they will be removed before submission}

% \begin{equation}
%         |x_{*}-\bar{x}_{*}| \leq \frac{\max_{\xi \in[x_{i}, x_{i+1}]} |f^{''}(\xi)|}{2U[i, i+1]}(x_{*}-x_{i})(x_{*}-x_{i+1})
% \end{equation}
% Let $s = x-x_{i}$
% \begin{equation}
%     (x_{*}-x_{i})(x_{*}-x_{i+1}) = s( s- h) = s^2 - sh
% \end{equation}

% \begin{equation}
%     2s - h = 0 \implies s = \frac{h}{2}
% \end{equation}
% substitute back
% \begin{equation}
%   s^2 - sh =\frac{h}{2}^{2} - \frac{h}{2}h = -\frac{h^{2}}{4} 
% \end{equation}
% \begin{equation}
%     |(x_{*}-x_{i})(x_{*}-x_{i+1})| = s^2 - sh \leq \frac{h^{2}}{4} \leq max \bigg(|x-\bar{x}_{*}|, |x-\bar{x}_{*}|\bigg)
% \end{equation}

%  \begin{figure*}[!htb]
%         \centering
%         %
%         \begin{subfigure}[b]{0.195 \textwidth}
%             \centering
%             \includegraphics[width= 0.99 \columnwidth]{figs/tangle_all_max_error128x128x128.png}
%             % \caption{Tangle}
%             \label{subfig:tangle_all_max_error}
%         \end{subfigure}
%         %%
%         \vspace{-9mm}
%         \begin{subfigure}[b]{0.195 \textwidth}
%             \centering
%             \includegraphics[width= 0.99 \columnwidth]{figs/torus_all_max_error128x128x128.png}
%             % \caption{Torus}
%             \label{subfig:torus_all_max_error}
%         \end{subfigure}
%         %%
%         \begin{subfigure}[b]{0.195 \textwidth}
%             \centering
%             \includegraphics[width= 0.99 \columnwidth]{figs/marschnerlobb_all_max_error128x128x128.png}
%             % \caption{Marschner and Lobb}
%             \label{subfig:marshnerlobb_all_max_error}
%         \end{subfigure}
%         %%
%         \begin{subfigure}[b]{0.195 \textwidth}
%             \centering
%             \includegraphics[width=0.99 \columnwidth]{figs/teardrop_all_max_error128x128x128.png}
%             % \caption{Teardrop}
%             \label{subfig:teardrop_all_max_error}
%         \end{subfigure}
%          %%
%         \begin{subfigure}[b]{0.195 \textwidth}
%             \centering
%             \includegraphics[width=0.99 \columnwidth]{figs/tubey_all_max_error128x128x128.png}
%             % \caption{Tubey}
%             \label{subfig:tubery_all_max_error}
%         \end{subfigure}
%         %%%%%%%%%%%%%%%%%%%%%%%%%%%%%%%%%%%%%%%%%%%%%%%%%%%%%%%%%%%%%%%%%%%%%%%%%%%%%%%%%%%%%%%%
%         %
%         \begin{subfigure}[b]{0.195 \textwidth}
%             \centering
%             \includegraphics[width= 0.99 \columnwidth]{figs/tangle_all_mean_error128x128x128.png}
%             % \caption{Tangle}
%             \label{subfig:tangle_all_mean_error}
%         \end{subfigure}
%         %%
%         \vspace{-9mm}
%         \begin{subfigure}[b]{0.195 \textwidth}
%             \centering
%             \includegraphics[width= 0.99 \columnwidth]{figs/torus_all_mean_error128x128x128.png}
%             % \caption{Torus}
%             \label{subfig:torus_all_mean_error}
%         \end{subfigure}
%         %%
%         \begin{subfigure}[b]{0.195 \textwidth}
%             \centering
%             \includegraphics[width= 0.99 \columnwidth]{figs/marschnerlobb_all_mean_error128x128x128.png}
%             % \caption{Marschner and Lobb}
%             \label{subfig:marshnerlobb_all_mean_error}
%         \end{subfigure}
%         %%
%         \begin{subfigure}[b]{0.195 \textwidth}
%             \centering
%             \includegraphics[width=0.99 \columnwidth]{figs/teardrop_all_mean_error128x128x128.png}
%             % \caption{Teardrop}
%             \label{subfig:teardrop_all_mean_error}
%         \end{subfigure}
%          %%
%         \begin{subfigure}[b]{0.195 \textwidth}
%             \centering
%             \includegraphics[width=0.99 \columnwidth]{figs/tubey_all_mean_error128x128x128.png}
%             % \caption{Tubey}
%             \label{subfig:tubery_all_mean_error}
%         \end{subfigure}
%         %%%%%%%%%%%%%%%%%%%%%%%%%%%%%%%%%%%%%%%%%%%%%%%%%%%%%%%%%%%%%%%%%%%%%%%%%%%%%%%%%%%%%%%%
%         %
%         \begin{subfigure}[b]{0.195 \textwidth}
%             \centering
%             \includegraphics[width= 0.99 \columnwidth]{figs/tangle_all_rms_error128x128x128.png}
%             \caption{Tangle}
%             \label{subfig:tangle_all_rms_error}
%         \end{subfigure}
%         %%
%         \begin{subfigure}[b]{0.195 \textwidth}
%             \centering
%             \includegraphics[width= 0.99 \columnwidth]{figs/torus_all_rms_error128x128x128.png}
%             \caption{Torus}
%             \label{subfig:torus_all_rms_error}
%         \end{subfigure}
%         %%
%         \begin{subfigure}[b]{0.195 \textwidth}
%             \centering
%             \includegraphics[width= 0.99 \columnwidth]{figs/marschnerlobb_all_rms_error128x128x128.png}
%             \caption{Marschner and Lobb}
%             \label{subfig:marschnerlobb_all_rms_error}
%         \end{subfigure}
%         %%
%         \begin{subfigure}[b]{0.195 \textwidth}
%             \centering
%             \includegraphics[width=0.99 \columnwidth]{figs/teardrop_all_rms_error128x128x128.png}
%             \caption{Teardrop}
%             \label{subfig:teardrop_all_rms_error}
%         \end{subfigure}
%          %%
%         \begin{subfigure}[b]{0.195 \textwidth}
%             \centering
%             \includegraphics[width=0.99 \columnwidth]{figs/tubey_all_rms_error128x128x128.png}
%             \caption{Tubey}
%             \label{subfig:tubery_all_rms_error}
%         \end{subfigure}
%         %%%%%%%%%%%%%%%%%%%%%%%%%%%%%%%%%%%%%%%%%%%%%%%%%%%%%%%%%%%%%%%%%%%%%%%%%%%%%%%%%%%%%%%%
%         \caption{Comparison of measured (in blue) and approximated error (in red).
%         %
%         The columns from left to right shows errors result for the Tangle (\autoref{subfig:tangle_all_rms_error}), Torus (\autoref{subfig:torus_all_rms_error}), Marschner and Lobb (\autoref{subfig:marschnerlobb_all_rms_error}), Teardrop (\autoref{subfig:teardrop_all_rms_error}), and Tubey (\autoref{subfig:tubery_all_rms_error}). }
%         \label{fig:figs_all_max_mean_rms}
%     \end{figure*}  

    
